# Supplementary material for: Generating Private Synthetic Data with Genetic Algorithms
Source: arXiv:2306.03257 source file (2023-06-05)
Supplement: Supplementary file 1 [file extra_prelims.tex]

% \section{Definitions}

% The notion of  zCDP enjoys a nice composition properties.
% \begin{lemma}[Composition]\label{lemma:composition}
%     Let $M:\mathcal{X}^n\rightarrow\mathcal{Y}$, and $M':\mathcal{X}^n\rightarrow\mathcal{Z}$ be randomized algorithms. Suppose $M$ satisfies $\rho$-zCDP and $M'$ satisfies $\rho'$-zCDP. Define $M'':\mathcal{X}^n\rightarrow\mathcal{Y}\times\mathcal{Z}$ by $M''(x)=(M(x),M'(x))$. Then $M''$ satisfies $(\rho+\rho')$-zCDP.
% \end{lemma}
